# Supplementary material for: tinyMAN: Lightweight Energy Manager using Reinforcement Learning for Energy Harvesting Wearable IoT Devices
Source: arXiv:2202.09297 source file (2022-03-18)
Supplement: Supplementary file 1 [file appendix.tex]

% \newpage
\setcounter{figure}{0}
\setcounter{equation}{0}
\section*{Appendix}
